# Supplementary material for: The N$^3$LO Twist-2 Matching of Helicity TMDs and SIDIS $q_\ast$ Spectrum
Source: arXiv:2509.01655 ancillary file (2026-09-10)
Supplement: Supplementary file 1 [file readme.pdf]

# Ancillary Files for “The N<sup>3</sup>LO Twist-2 Matching of Helicity TMDs and SIDIS $q_*$ Spectrum”

Yu Jiao Zhu<sup>1,\*</sup>

<sup>1</sup>*Zhejiang Institute of Modern Physics, Department of Physics, Zhejiang University, Hangzhou, 310027, China*

In this note we explain the definitions and conventions for the ancillary files associated with the arXiv submission of “The N<sup>3</sup>LO Twist-2 Matching of Helicity TMDs and SIDIS  $q_*$  Spectrum”.

## FLAVOR DECOMPOSITION

In this section, we fix our notations for flavor group decomposition of the coefficient functions, the PDFs (FFs) and the splitting functions. We begin with the non-singlet sectors, denoting  $q$  to be a quark,  $\bar{q}$  an anti-quark and  $q'$  another flavor of quark, the ‘valence’ quark contributions are defined as ( $f$  can be identified as partonic PDFs, the coefficient functions or the splitting functions of some flavor)

$$f_{qq}^v = f_{qq} - f_{qq'}, \quad f_{q\bar{q}}^v = f_{q\bar{q}} - f_{q\bar{q}'} . \quad (1)$$

By linear combinations, we define three independently evolving types of non-singlets

$$\begin{aligned} f_{ns}^+ &= f_{qq}^v + f_{q\bar{q}}^v, & f_{ns}^- &= f_{qq}^v - f_{q\bar{q}}^v, \\ f_{ns}^v &= f_{ns}^- + N_f(f_{qq'} - f_{q\bar{q}'}), \end{aligned} \quad (2)$$

note that the ‘sea’ quark difference  $f_{qq'} - f_{q\bar{q}'}$  vanishes up to  $\alpha_s^2$ , and is non-vanishing from the third order. In particular, we denote the ‘sea’ quark difference as

$$f_{d_{abc}^2} = N_f(f_{qq'} - f_{q\bar{q}'}), \quad (3)$$

since at 3-loop, they are proportional to the cubic color structure  $d_{abc}^2$ . For the singlet sector, we define

$$\begin{aligned} f_{qq}^s &= f_{ns}^+ + N_f(f_{qq'} + f_{q\bar{q}'}), & f_{qq}^s &\equiv f_{ns}^+ + f_{qq}^{ps}, \\ f_{q\bar{q}}^s &= 2N_f f_{q\bar{q}}, & f_{q\bar{q}}^s &= f_{q\bar{q}}, & f_{gq}^s &= f_{gq}, & f_{g\bar{q}}^s &= f_{g\bar{q}}. \end{aligned} \quad (4)$$

In the ancillary files, the flavor index ‘ps’ (the pure singlet sector, i.e. the sum of all sea quarks) and the flavor index ‘ $d_{abc}^2$ ’ (the ‘sea’ quark difference at 3-loop) are extensively used. Their incorporation into the singlet sector (denoted as ‘s’) and the non-singlet sector with flavor index ‘v’ can be found in Eq. 2, Eq. 3 and Eq. 4.

## SCHEME DEPENDENCE

Our results for the splitting functions and the coefficient functions depend on the prescription of  $\gamma_5$  in dimensional regularization, expressions in different schemes are related by scheme transformation factors. The transformation factors are defined with respect to the flavor

group, for flavor group index  $i = \pm, v, s$  and in Mellin-N space, they allow perturbative expansions of the form

$$Z_i = 1 + \sum_n \left( \frac{\alpha_s}{4\pi} \right)^n z_i^{(n)}. \quad (5)$$

In the singlet sector with  $i = s$ , the transformation factors are  $2 \times 2$  matrices in Mellin-N space, but the matrix elements are nontrivial only in the  $q \rightarrow q$  channel, indeed we have (here ns = +)

$$(z_s^{(n)})_{ik} = \delta_{iq} \delta_{kq} z_{qq}^{(n)} = \delta_{iq} \delta_{kq} \left\{ z_{ns}^{(n)} + z_{ps}^{(n)} \right\}. \quad (6)$$

In this paper, we consider transformation rules between  $\overline{MS}$  and HVBM (denoted as ‘L’) scheme. For the coefficient functions, the transformation rules are

$$\Delta \mathcal{I}_{\overline{MS}}^i = \Delta \mathcal{I}_L \otimes Z_i^{-1}, \quad \Delta \mathcal{I}_{\overline{MS}}^i = (Z_i^T)^{-1} \otimes \Delta \mathcal{C}_L, \quad (7)$$

where  $i = \pm, v, s$  are flavor group indices.

For the splitting functions, we define their differences as  $\delta[\Delta P] = \Delta P_{\overline{MS}} - \Delta P_L$ . In the non-singlet sectors with ns=±, v, we have

$$\begin{aligned} \delta[\Delta P_{ns}] &= \left( \frac{\alpha_s}{4\pi} \right)^2 \left\{ -\beta_0 z_{ns}^{(1)} \right\} + \left( \frac{\alpha_s}{4\pi} \right)^3 \left\{ \beta_0 \left( z_{ns}^{(1)} \right)^2 \right. \\ &\quad \left. - \beta_1 z_{ns}^{(1)} - 2\beta_0 z_{ns}^{(2)} \right\} + \mathcal{O}(\alpha_s^4), \\ \delta[\Delta P_{ns}^T] &= \left( \frac{\alpha_s}{4\pi} \right)^2 \left\{ -\beta_0 z_{ns}^{T(1)} \right\} + \left( \frac{\alpha_s}{4\pi} \right)^3 \left\{ \beta_0 \left( z_{ns}^{T(1)} \right)^2 \right. \\ &\quad \left. - \beta_1 z_{ns}^{T(1)} - 2\beta_0 z_{ns}^{T(2)} \right\} + \mathcal{O}(\alpha_s^4). \end{aligned} \quad (8)$$

For the singlet sectors, the transformation rules for the space-like splitting functions read

$$\begin{aligned} \delta[\Delta P_{qq}^{s(1)}] &= -\beta_0 z_{qq}^{(1)}, & \delta[\Delta P_{q\bar{q}}^{s(1)}] &= z_{q\bar{q}}^{(1)} \otimes \Delta P_{q\bar{q}}^{s(0)} \\ \delta[\Delta P_{gq}^{s(1)}] &= -\Delta P_{gq}^{s(0)} \otimes z_{q\bar{q}}^{(1)}, & \delta[\Delta P_{g\bar{q}}^{s(1)}] &= 0, \end{aligned} \quad (9)$$

and

$$\begin{aligned} \delta[\Delta P_{qq}^{s(2)}] &= \beta_0 \left[ \left( z_{qq}^{(1)} \right)^2 - 2z_{qq}^{(2)} \right] - \beta_1 z_{qq}^{(1)}, \\ \delta[\Delta P_{q\bar{q}}^{s(2)}] &= z_{q\bar{q}}^{(2)} \otimes \Delta P_{q\bar{q}}^{s(0)} + z_{q\bar{q}}^{(1)} \otimes \Delta P_{q\bar{q},L}^{s(1)}, \\ \delta[\Delta P_{gq}^{s(2)}] &= - \left( \Delta P_{gq,L}^{s(1)} - \Delta P_{gq}^{s(0)} \otimes z_{q\bar{q}}^{(1)} \right) \otimes z_{q\bar{q}}^{(1)} \\ &\quad - \Delta P_{gq}^{s(0)} \otimes z_{q\bar{q}}^{(2)}, \\ \delta[\Delta P_{g\bar{q}}^{s(2)}] &= 0, \end{aligned} \quad (10)$$

and the transformation rules for the singlet time-like splitting functions read

$$\begin{aligned}\delta[\Delta P_{qq}^{T,s(1)}] &= -\beta_0 z_{qq}^{T(1)}, \quad \delta[\Delta P_{gq}^{T,s(1)}] = z_{qq}^{T(1)} \otimes \Delta P_{gq}^{T,s(0)} \\ \delta[\Delta P_{qg}^{T,s(1)}] &= -\Delta P_{qg}^{T,s(0)} \otimes z_{qq}^{T(1)}, \quad \delta[\Delta P_{gg}^{T,s(1)}] = 0,\end{aligned}\quad (11)$$

and

$$\begin{aligned}\delta[\Delta P_{qq}^{T,s(2)}] &= \beta_0 \left[ \left( z_{qq}^{T(1)} \right)^2 - 2z_{qq}^{T(2)} \right] - \beta_1 z_{qq}^{T(1)}, \\ \delta[\Delta P_{gq}^{T,s(2)}] &= z_{qq}^{T(2)} \otimes \Delta P_{gq}^{T,s(0)} + z_{qq}^{T(1)} \otimes \Delta P_{gq,L}^{T,s(1)}, \\ \delta[\Delta P_{qg}^{T,s(2)}] &= - \left( \Delta P_{qg,L}^{T,s(1)} - \Delta P_{qg}^{T,s(0)} \otimes z_{qq}^{T(1)} \right) \otimes z_{qq}^{T(1)} \\ &\quad - \Delta P_{qg}^{T,s(0)} \otimes z_{qq}^{T(2)}, \\ \delta[\Delta P_{gg}^{T,s(2)}] &= 0.\end{aligned}\quad (12)$$

The 3-loop transformation factors are collected in the file `z5SL.m` for the space-like ones and in the file `z5TL.m` for the time-like ones. For  $i = \pm$

$$\text{Z5}["i"] = \delta(1-z) + \sum_{n=1}^{n=3} \left( \frac{\alpha_s}{4\pi} \right)^n z_i^{(n)}(z), \quad (13)$$

where  $\delta(1-z)$  is the Dirac delta function. And for  $i = \text{ps}$

$$\text{Z5}["\text{ps}"] = \left( \frac{\alpha_s}{4\pi} \right)^2 z_{\text{ps}}^{(2)}(z) + \left( \frac{\alpha_s}{4\pi} \right)^3 z_{\text{ps}}^{(3)}(z). \quad (14)$$

For user's convenience, we also have the inverse of the transformation factors with function head `inverseZ5["i"]`.

### SPACE-LIKE TMD HELICITY DISTRIBUTION FUNCTION

In the MATHEMATICA file `dBeamMSb.m` and `dBeamLarin.m`, we provide matching coefficients for the space-like TMD helicity distribution functions in  $\overline{\text{MS}}$  and HVBM scheme, respectively, the space-like coefficient functions are known as ‘beam functions’. In the non-singlet sectors with  $i = \pm, d_{abc}^2$ , we use function head `dBeamMSb["i"]` (`dBeamLarin["i"]`). In the singlet sector, we use function head `dBeamMSb["ji"]` (`dBeamLarin["ji"]`), where  $i$  or  $j$  can be either quark or gluon. Our results are expanded in terms of the strong coupling  $\text{as} = \frac{\alpha_s(\mu)}{4\pi}$ , for the example of the singlet sector we have

$$\begin{aligned}\text{dBeamMSb}["ji"] &= \Delta \mathcal{I}_{ji}^{s(0)} + \text{as} \Delta \mathcal{I}_{ji}^{s(1)} + \text{as}^2 \Delta \mathcal{I}_{ji}^{s(2)} \\ &\quad + \text{as}^3 \Delta \mathcal{I}_{ji}^{s(3)}.\end{aligned}\quad (15)$$

The logarithmic terms in these files are defined by

$$\text{Lp} = L_\perp = \ln(|b_\perp^2| \mu^2 / b_0^2), \quad \text{LQ} = L_Q = 2 \ln(Q/\nu), \quad (16)$$

where  $Q = xP^+$  is the momenta flow (twice the energy of the active parton) into the hard scattering processes.

‘Beam functions’ are rapidity regulator independent, in particular they depend on the rapidity scale  $\nu$ . Rapidity-regulator-independent TMD helicity PDFs are obtained by multiplying the beam functions with the square root of the soft functions

$$\Delta \mathcal{J}_{ij}(x, b_\perp, P^+, \mu) = \Delta \mathcal{I}_{ij}(x, b_\perp, P^+, \mu, \nu) \sqrt{\mathcal{S}_i(b_\perp, \mu, \nu)}. \quad (17)$$

Note that for  $i = q, g$  in Eq. (17),  $\mathcal{S}_q$  and  $\mathcal{S}_g$  are related by Casimir scaling up to 3-loop. In the files `dPDFMSb.m` and `dPDFLarin.m`, we collect the results for the TMD helicity PDFs, where we use function head `dPDFMSb["i"]` (`dPDFLarin["i"]`) for the non-singlet sectors ( $i = \pm, d_{abc}^2$ ), and function head `dPDFMSb["ij"]` (`dPDFLarin["ij"]`) for the singlet sector, everything proceeds in parallel with the case of beam functions, except for the introduction of the Collins-Soper scale logarithm

$$\text{Lh} = L_\nu + L_Q = \ln(Q^2/\mu^2). \quad (18)$$

To facilitate numerical implementation, the numerical fits in the files `dBeamMSbN.m` and `dPDFMSbN.m` are also provided.

### TIME-LIKE TMD HELICITY FRAGMENTATION FUNCTION

In the MATHEMATICA file `dFragMSb.m` and `dFragLarin.m`, we provide matching coefficients for the time-like TMD helicity fragmentation functions. In the non-singlet sectors with  $i = \pm, d_{abc}^2$ , we use function head `dFragMSb["i"]` (`dFragLarin["i"]`). In the singlet sector, we use function head `dFragMSb["ji"]` (`dFragLarin["ji"]`), where  $i$  or  $j$  can be either quark or gluon. Our results are expanded in terms of the strong coupling  $\text{as} = \frac{\alpha_s(\mu)}{4\pi}$ , for the example of the singlet sector we have

$$\begin{aligned}\text{dFragMSb}["ji"] &= \Delta \mathcal{C}_{ji}^{s(0)} + \text{as} \Delta \mathcal{C}_{ji}^{s(1)} + \text{as}^2 \Delta \mathcal{C}_{ji}^{s(2)} \\ &\quad + \text{as}^3 \Delta \mathcal{C}_{ji}^{s(3)}.\end{aligned}\quad (19)$$

The logarithmic terms in these files are defined by

$$\text{Lp} = L_\perp = \ln(|b_\perp^2| \mu^2 / b_0^2), \quad \text{LQ} = L_Q = 2 \ln(Q/\nu), \quad (20)$$

where  $Q = P^+/z$  is twice the energy of the fragmentaed parton.

Rapidity-regulator-independent TMD helicity FFs are obtained by multiplying the time-like coefficient functions with the square root of the soft functions, the soft

functions used in the time-like case here are identical to those of space-like ones up to  $\alpha_s^3$ .

$$\Delta\mathcal{C}_{ij}(z, b_\perp, P^+, \mu) = \Delta\mathcal{C}_{ij}(z, b_\perp, P^+, \mu, \nu) \sqrt{\mathcal{S}_j(b_\perp, \mu, \nu)}. \quad (21)$$

In the files `dFFMSb.m` and `dFFLarin.m`, we collect the results for the TMD helicity FFs, where we use function head `dFFMSb["i"]` (`dFFLarin["i"]`) for the non-singlet sectors ( $i = \pm, d_{abc}^2$ ), and function head `dFFMSb["ij"]` (`dFFLarin["ij"]`) for the singlet sector. The Collins-Soper scale logarithm appeared in the expressions of the TMD helicity FFs is defined by

$$L_h = L_\nu + L_Q = \ln(Q^2/\mu^2). \quad (22)$$

To facilitate numerical implementation, the numerical fits in the file `dFragMSbN.m` and `dFFMSbN.m` are also provided.

### TMD SOFT FUNCTION

The MATHEMATICA file `softfunction.m` gives the quark TMD soft function to N<sup>3</sup>LO with

$$L_\nu = L_\nu = \ln(\nu^2/\mu^2). \quad (23)$$

Expressions for gluon TMD function is easily obtained by Casimir scaling. The soft zero-bin function is identical to TMD soft function and is universal for both space-like and time-like configurations up to  $\mathcal{O}(\alpha_s^3)$ .

### SYMBOLS AND COLORS

For the color factors,

$$\begin{aligned} \text{CF} &= C_F, \quad \text{Nf} = N_f, \quad \text{TF} = T_F, \quad \text{CA} = C_A, \\ \frac{\text{dabc2}}{\text{nc}} &= \frac{d^{ABC} d_{ABC}}{N_c} = \frac{(N_c^2 - 1)(N_c^2 - 4)}{N_c^2}. \end{aligned} \quad (24)$$

`plusD[n, 1-z]` is the conventional plus distribution

$$\text{plusD}[n, 1-z] = \left( \frac{\ln^n(1-z)}{1-z} \right)_+. \quad (25)$$

Dirac delta function is represented by

$$\text{delta}[1-z] = \delta(1-z).$$

Harmonic polylogarithms are represented by

$$H[\mathbf{a1}, \mathbf{a2}, \dots, \mathbf{an}, \mathbf{z}] = \text{HPL}[\{\mathbf{a1}, \mathbf{a2}, \dots, \mathbf{an}\}, \mathbf{z}],$$

and `zeta[n]` is Riemann zeta value  $\zeta_n$ .

When referring to the results calculated in this paper, please kindly cite Refs. [1, 2].

---

\* zhuyujiao@zju.edu.cn

- [1] Y.J. Zhu, “The N<sup>3</sup>LO Twist-2 Matching of Helicity TMDs and SIDIS  $q_*$  Spectrum,” [arXiv:25??xxxx [hep-ph]].
- [2] Y. Li and H. X. Zhu, “Bootstrapping Rapidity Anomalous Dimensions for Transverse-Momentum Resummation,” Phys. Rev. Lett. **118**, no. 2, 022004 (2017) [arXiv:1604.01404 [hep-ph]].
